# Supplementary material for: Beyond Words: Augmenting Discriminative Richness via Diffusions in Unsupervised Prompt Learning
Source: arXiv:2504.11930 source file (2025-04-16)
Supplement: Supplementary file 1 [file 6_supp.tex]

\section{Overall Algorithm}
We present the comprehensive algorithmic flow of the AiR method in Algorithm~\ref{al:wa}.
To balance data diversity and domain consistency in augmented images, we first fine-tune the SD model using LoRA. Subsequently, synthetic images $\hat{X}$ are generated via the fine-tuned Stable Diffusion Model (SD), and the samples most aligned with the semantic information are selected based on cosine similarity. The chosen synthetic images $\hat{X}^*$ serve as auxiliary classifiers, working alongside text classifiers to assign pseudo-labels $\tilde{y}^*$ to the unlabeled samples. Finally, the pseudo-labeled data $(x, \tilde{y}^*)$ and synthetic data $(\hat{x}, y)$  are used as training samples to compute the loss and iteratively optimize the prompt.

\begin{algorithm}
    \SetAlgoLined
    \caption{Workflow about our AiR method for optimizing prompt $t$}
    \label{al:wa}
    \SetKwInOut{Input}{Input}
    \SetKwInOut{Output}{Output}
    Get pseudo label data $\{x, \tilde{y}\}$ in Eq. (2) \\
    Finetune SD with LoRA in Eq. (4) \\ 
    Generate synthetic images $\hat{X}$ in Eq. (5) \\
    Select high confidence samples $\hat{X}^*$ \\
    \For{$iter=1,2,3,...$}{
    Text-image prediction
    $p_c = \frac{\text{exp}(\text{sim}({f}, {g}_c) / \tau)}{\sum_{c^{\prime}=1}^C \text{exp}(\text{sim}({f}, {g}_{c^{\prime}}) / \tau)}$ \\
    Image-image prediction
    $\hat{p}_c = \frac{\text{exp}(\text{sim}({f}, \hat{x}_c^*) / \tau)}{\sum_{c^{\prime}=1}^C \text{exp}(\text{sim}({f}, \hat{x}_{c^{\prime}}^*) / \tau)}$ \\
    Combine both types of predictions
    $p_c^* = p_c + \lambda * \hat{p}_c$ \\
    Pseudo labels $\tilde{y}^* = \underset{c} {\text{argmax}}p_c^*$ \\
    Real data loss $\underset{t}{\text{min}}\mathcal{L}_{r} = \underset{t}{\text{min}}\mathcal{L}_{ce}(x, \tilde{y}^*)$ \\
    Synthetic data loss $\underset{t}{\text{min}}\mathcal{L}_{s} = \underset{t}{\text{min}}\mathcal{L}_{ce}(\hat{x}, y)$ \\
    Total loss $\underset{t}{\text{min}}\mathcal{L} = \underset{t}{\text{min}}(\mathcal{L}_{r} + \beta * \mathcal{L}_{s})$ \\
    Take gradient descent step on
    $\nabla \mathcal{L}$ \\
    Update $t^{iter+1} \leftarrow t^{iter} - \eta \nabla \mathcal{L}$ \\
    }
\end{algorithm}

\begin{table}[!t]
\centering

\resizebox{.45\textwidth}{!}{
\begin{tabular}{l c c c}
	\toprule
      Method & RESISC45  & EuroSAT & DTD \\ 
      \hline
      % Cosine Distance & & & \\
      Kandinsky2.2 & 77.6 & 69.5  & 54.3 \\
      Dreambooth &  78.3 & 70.8 &  54.8    \\
      \rowcolor{gray!15}
      Stable Diffusion & \textbf{79.9} &  \textbf{71.4} &  \textbf{55.7}  \\
      % \hline
%      Cross-entropy pipeline & 57.7 & 88.6 & 81.6 & 80.5 & 67.7  \\ 
      % Ours & 130.2202 & 4.2388 & 21.00  \\
	\bottomrule
\end{tabular}}
\caption{
Comparison of top-1 test accuracy ($\%$) in unsupervised learning with different generative models: Kandinsky2.2, Dreambooth, and Stable Diffusion.
The best results are in \textbf{bold}.
}
\label{tab:gen}
% \vspace{-10pt}
\end{table}

\section{Task Introduction}
We outline the experimental settings for three distinct learning paradigms following~\cite{menghini2023enhancing, zhang2024candidate}:

\noindent\textbf{Semi-Supervised Learning (SSL)}: In this paradigm, access to labeled data is restricted. 
To evaluate the influence of pseudo-labels, we consider scenarios with minimal labeled data and abundant unlabeled data, using two labeled samples per class.

\noindent\textbf{Unsupervised Learning (UL)}: Here, only unlabeled data is available. 
Pseudo-labels are initially derived entirely from the zero-shot predictions of CLIP, eliminating the need for any manual annotation.

\noindent\textbf{Transductive Zero-Shot Learning (TRZSL)}: In this setting, labeled data is provided for a subset of target classes (seen classes) in the downstream dataset. 
We set the seen-to-unseen class ratio to 62:38, with pseudo-labels generated exclusively for unseen classes. 
Additionally, for TRZSL, we report the harmonic mean of the accuracies for seen and unseen classes to account for performance balance.

\section{Finetune with LoRA}
We fine-tune the Stable Diffusion-v1-4 (SD) model using LoRA~\cite{hu2022lora}, following the approach in~\cite{von-platen-etal-2022-diffusers}.
For each dataset, we select the top 5 pseudo-labeled samples with the highest confidence to train the SD model.
To ensure alignment between the SD model and the semantic space of CLIP's text encoder, only the U-Net component of SD is fine-tuned.
The model is trained for 15,000 steps with a batch size of 1, using a learning rate of 1e-5.

\section{Effect of Generative Models}
To investigate the performance variations of our AiR method across different generative models, we fine-tune three models: Kandinsky 2.2, DreamBooth~\cite{ruiz2023dreambooth}, and Stable Diffusion using LoRA and apply the same training strategy for the AiR model, with CPL as the baseline.
As shown in Table~\ref{tab:gen}, we conduct experiments on three datasets, and the results indicate that the performance of AiR across these generative models varies by less than 2\%. 
This demonstrates that our method is not heavily dependent on the choice of the generative model, as long as the model can be fine-tuned to ensure both the fidelity of the generated images and sample diversity. 
However, DreamBooth requires individual fine-tuning for each category, leading to higher computational costs, while Kandinsky 2.2 shows slightly lower performance compared to Stable Diffusion. 
Consequently, we select Stable Diffusion as the generative model for our AiR framework.

\section{Effect of Cosine Selected Strategy}
To determine the most effective filtering strategy for selecting representative synthetic samples, we evaluate different similarity metrics between synthetic samples and textual features across three datasets. We report the pseudo-labeling accuracies of the Top-50 confidence samples for the CLIP model after incorporating synthetic samples as auxiliary classifiers.
As shown in Table~\ref{tab:cos}, we test the Euclidean distance, OT distance~\cite{villani2009optimal}, and cosine similarity. The Euclidean distance results in a significant drop in performance, indicating its unsuitability for selecting synthetic samples. Both OT distance and cosine similarity demonstrate comparable performance, with a slight degradation observed for OT distance. Considering that OT distance requires higher computational resources compared to cosine similarity, we ultimately select cosine similarity as the filtering strategy to identify the most representative synthetic samples.

\begin{table}[!t]
\centering

\resizebox{.45\textwidth}{!}{
\begin{tabular}{l c c c }
	\toprule
      Method & Flowers102  & DTD & EuroSAT \\ 
      \hline
      % Cosine Distance & & & \\
      Euclidean Distance &  54.8 & 51.5 &  73.0 \\
      OT distance & 68.3 & 62.3 & 76.6 \\
      \rowcolor{gray!15}
      Cosine Distance & \textbf{68.3} &  \textbf{62.3} &  \textbf{76.6}  \\
      % \hline
%      Cross-entropy pipeline & 57.7 & 88.6 & 81.6 & 80.5 & 67.7  \\ 
      % Ours & 130.2202 & 4.2388 & 21.00  \\
	\bottomrule
\end{tabular}}
\caption{
Comparison of top-1 test accuracy ($\%$) in unsupervised learning with different similarity metrics: Euclidean Distance, OT distance, and Cosine Distance.
The best results are in \textbf{bold}.
}
\label{tab:cos}
% \vspace{-10pt}
\end{table}

\section{Hyper-parameters}
To investigate the influence of hyperparameters $\lambda$ and $\beta$ discussed in Sec. 3.5, we evaluate the accuracy of pseudo-labels by varying their values on the EuroSAT~\cite{helber2019eurosat} and RESISC45~\cite{cheng2017remote} datasets.
As illustrated in Fig.~\ref{fig:lamada} and Fig.~\ref{fig:beta}, the model's accuracy fluctuates by approximately 3\% when $\lambda$ changes from 1/8 to 1. This suggests that effectively balancing the results of the auxiliary classifier (constructed using synthetic samples) and the text classifier is crucial. Overemphasizing either side diminishes the quality of the pseudo-labels. We observe optimal performance when $\lambda$ is set to 1/6 or 1/4, achieving 78.6\% accuracy on the EuroSAT dataset and 83.8\% on the RESISC45 dataset. Consequently, for our final experiments, we select $\lambda$ as 1/6.
Similarly, when adjusting $\beta$ between 1/4 and 2, the model's performance remains relatively stable. This indicates that optimizing the network with synthetic samples as a loss function does not require extensive fine-tuning of $\beta$. Ultimately, we choose 1 as the value of $\beta$ for its higher performance consistency.

\begin{figure}
\centering

\includegraphics[width=.9\linewidth]{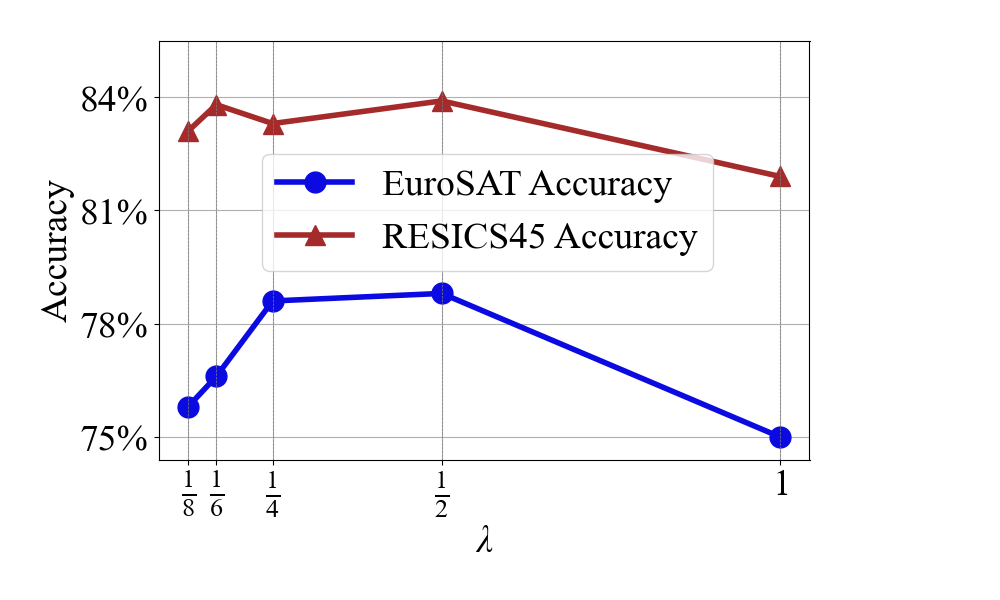}
% \vspace{-5pt}
\caption{
Comparison of top-1 test accuracy ($\%$) of pseudo labels with different hyper-parameters $\lambda$. 
% `Ours' denotes the use of our approach AiR, while `CLIP' indicates the use of only CLIP's text encoder.
}
% \vspace{-20pt}
\label{fig:lamada}
\end{figure}
\begin{figure}
\centering

\includegraphics[width=.9\linewidth]{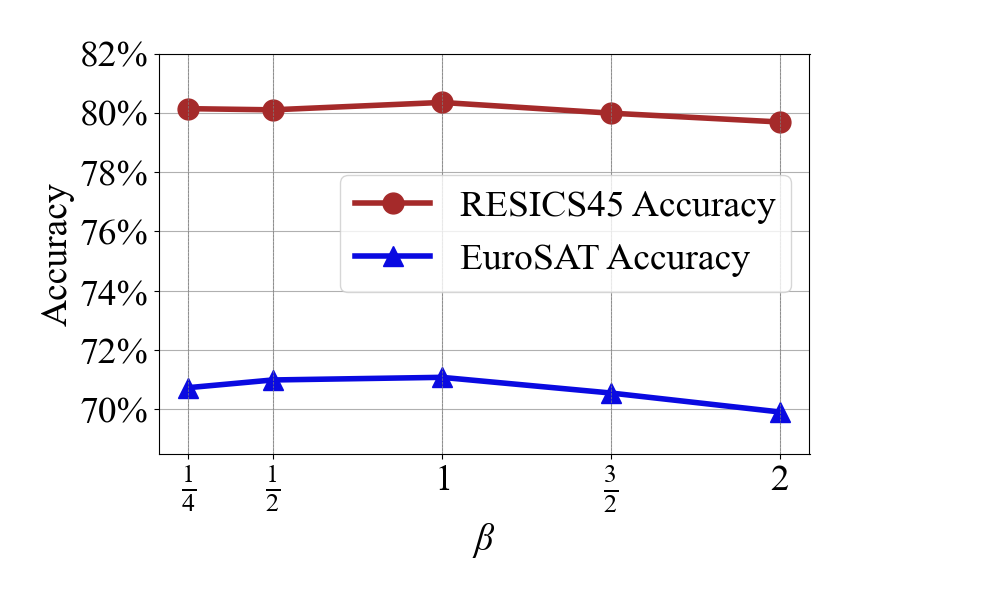}
% \vspace{-5pt}
\caption{
Comparison of top-1 test accuracy ($\%$) of pseudo labels with different hyper-parameters $\beta$.
}
% \vspace{-20pt}
\label{fig:beta}
\end{figure}

\section{Pseudo Label Accuracy}
To further illustrate the impact of our method on enhancing pseudo-labeling quality, we compare the pseudo-labeling accuracy of CPL (used as a baseline) with that of our AiR method on the Flowers102~\cite{nilsback2008automated} dataset over successive training iterations.
As depicted in Fig.~\ref{fig:plaa}, the pseudo-labeling accuracy of our method consistently surpasses that of the baseline by 2\%-7\% as training progresses. 
This highlights the sustained improvement in pseudo-labeling quality achieved by our approach. 
The stable accuracy margin of over 2\% further validates that our method generates high-quality pseudo-labeled samples, enabling the training of a more robust unsupervised prompt learning model.

\begin{figure}
\centering

\includegraphics[width=.9\linewidth]{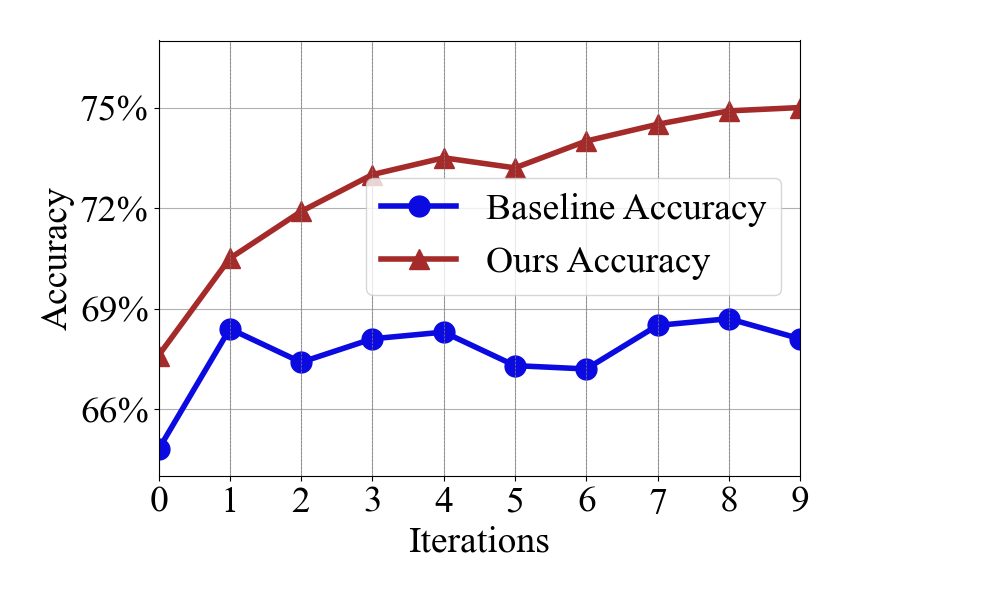}
% \vspace{-5pt}
\caption{
Comparison of top-1 test accuracy ($\%$) of pseudo labels during different training iterations.
}
% \vspace{-15pt}
\label{fig:plaa}
\end{figure}

\section{t-SNE of Different Discrimination Outcomes.}
In this section, we analyze the spatial distribution of synthetic image embeddings, text embeddings, and sample embeddings using t-SNE visualizations on the DTD and RESISC45 datasets.
As illustrated in Fig.~\ref{fig:tsdtd} and Fig.~\ref{fig:tsres}, colored circular dots represent different image classes, triangles indicate the text embeddings for each class, squares denote the synthetic image embeddings, and pentagrams represent the fused embeddings of text and synthetic images, as described in Sec. 3.5.
The findings are consistent with the results discussed in the main paper. 
The fused embeddings (pentagrams) reveal a clear tendency for text embeddings to shift toward their corresponding test sample classes. 
This alignment indicates that augmenting discriminative information effectively calibrates the embeddings, bringing them closer to the correct test samples and enhancing the model’s classification accuracy across various classes.

\begin{figure}
\centering

\includegraphics[width=.9\linewidth]{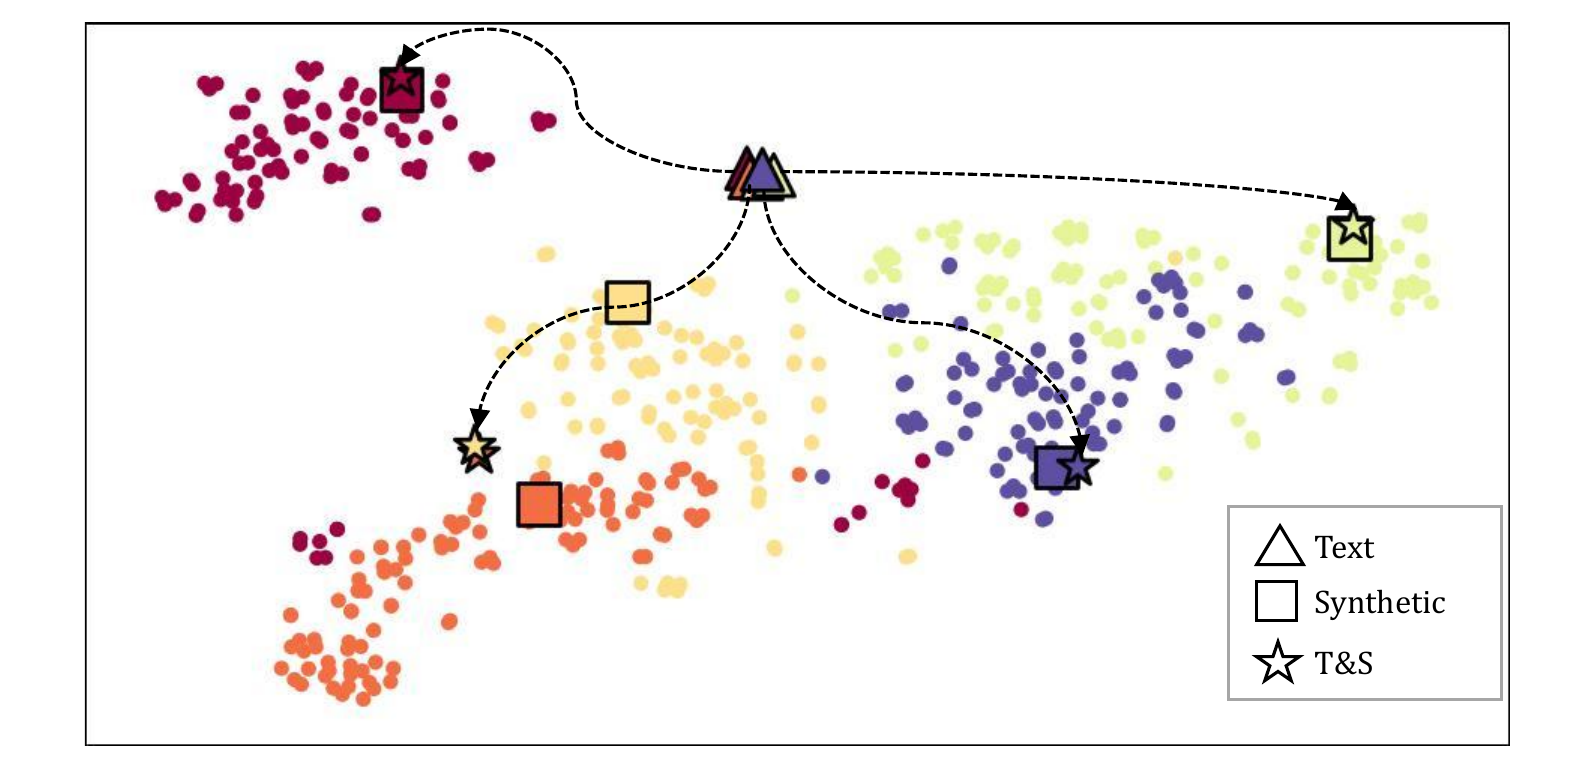}
% \vspace{-5pt}
\caption{
Visualization of the spatial distribution of synthetic image, text, and sample embeddings
with t-SNE in DTD dataset.
}
% \vspace{-20pt}
\label{fig:tsdtd}
\end{figure}

\begin{figure}
\centering

\includegraphics[width=.9\linewidth]{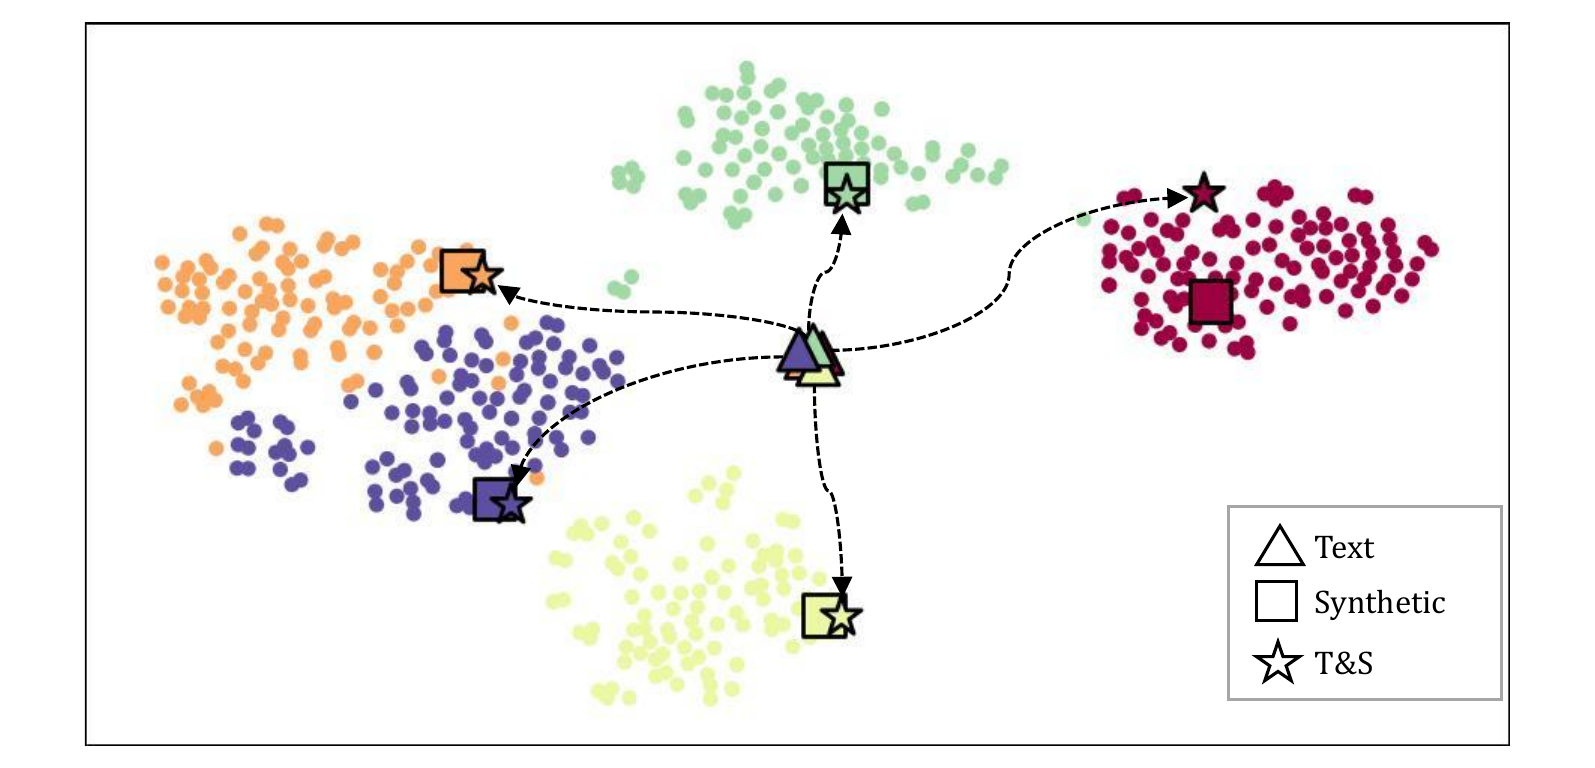}
% \vspace{-5pt}
\caption{
Visualization of the spatial distribution of synthetic image, text, and sample embeddings
with t-SNE in RESISC45 dataset.
}
% \vspace{-20pt}
\label{fig:tsres}
\end{figure}

\section{Comparison on Large Scale Dataset.}
We conduct experiments on ImageNet, which is challenging and not considered by other works.
Due to memeory constraints, we select 100 samples per class.
As shown in Table~\ref{tab:r1a3}, ours outperforms CPL by nearly 2\% accuracy. 
These results indicate that our AiR consistently boosts the classification performance of prompt learning models even on large scale dataset, demonstrate the robustness of our method.

\begin{table}[!t]
\centering

\resizebox{.35\textwidth}{!}{
\begin{tabular}{c c c c }
\toprule
 Method  & &ImageNet & \\
   & SSL & UL  & TRZSL \\ 
\hline
CPL & 61.6 & 62.8  &  65.3 \\ 
\rowcolor{gray!15}
Ours & \textbf{63.9}  & \textbf{64.9}  &  \textbf{67.2} \\ 
\bottomrule
\end{tabular}
}

\caption{Comparison results of top-1 test accuracy (\%) on ImageNet dataset.
The best results are in \textbf{bold}.
}

\label{tab:r1a3}
% \vspace{-20pt}
\end{table}
% We will include more baselines in the revision.

\section{Comparison in Cross-dataset Scenarios.}
To further demonstrate the generalisability of our approach, we perform comparative experiments in cross-dataset scenarios.
We train models on RESISC45/Flowers102/DTD and test them on other datasets. 
As shown in Tab.~\ref{tab:r3a5}, our Air still surpasses the SOTA-CPL by \textbf{3-8\%} accuracy, proving its generalizability.

\begin{table}[!t]
\centering
\resizebox{.45\textwidth}{!}{
\begin{tabular}{l  c | c c c c c}
	\toprule
      Method  & Source  &  & & Target & & \\
       &RESISC45 &Flowers102 &FGVCaircraft &DTD &EuroSAT  & Average\\
    \hline
    CPL & 77.3 & 36.2 & 2.6 & 16.9 & 35.3  & 22.7 \\
    \rowcolor{gray!15}
    Ours &  \textbf{79.9} & \textbf{49.6} & \textbf{6.9} & \textbf{24.3} & \textbf{44.5} & \textbf{31.3} \\ 
    \hline
     &Flowers102  &RESISC45  &FGVCaircraft &DTD &EuroSAT  & Average\\
    \hline
    CPL & 72.9 & 20.4 & 6.3 & 20.9 & 34.7 & 20.5 \\
    \rowcolor{gray!15}
    Ours &  \textbf{74.3} & \textbf{28.4} & \textbf{6.5} & \textbf{29.3} & \textbf{39.9} & \textbf{26.0} \\ 
    \hline
     &DTD  &RESISC45  &FGVCaircraft &Flowers102 &EuroSAT  & Average\\
    \hline
    CPL & 51.9 & 40.8 & 4.4 & 45.7 & 27.5 & 29.6 \\
    \rowcolor{gray!15}
    Ours &  \textbf{55.7} & \textbf{44.3} & \textbf{5.2} & \textbf{47.9} & \textbf{32.5} & \textbf{32.5} \\ 
    \bottomrule
\end{tabular}
}
%}
\caption{
Results in cross-dataset scenarios.
}
% \vspace{-20pt}
\label{tab:r3a5}
% }
\end{table}
